# Supplementary material for: High-temperature observation of intralayer, interlayer, and Rydberg excitons in bulk van der Waals alloy single crystals
Source: arXiv:2408.16306 source file (2024-08-29)
Supplement: Supplementary file 1 [file SM.pdf]

Supplemental Material

# High-temperature observation of intralayer, interlayer, and Rydberg excitons in bulk van der Waals alloy single crystals

Pravrati Taank[1], Asif Ali[1], Aravind Raji[1], Ajay K. Poonia[1], Matthew C. Beard[2], Ravi Shankar Singh[1*], and K. V. Adarsh[1*]

[1]*Department of Physics, Indian Institute of Science Education and Research, Bhopal 462066, India*

[2]*Chemistry & Nanoscience Center, National Renewable Energy Laboratory; Golden, Colorado 80401, USA*

**Corresponding Author***

Email: rssingh@iiserb.ac.in and adarsh@iiserb.ac.in

**Contents:**

S1. Comparison with previous studies 2

S2. Structural and compositional properties of bulk alloy single crystals 3-7

S3. Theoretical calculations 8-9

S4. Angle-resolved photoemission spectroscopy (ARPES) 10-11

S5. Crystal structure 12

S6. Temperature-dependent reflectance spectroscopy 13

S7. Rydberg excitons in bulk alloy single crystals 14

S8. Assignment of A' and B' excitonic transitions 15

S9. Intra and interlayer excitons in TMDs 16

S10. Calculated absorption spectrum for monolayer alloys 17

S11. Phonon dispersion curves of bulk alloys 18

References 19

## S1. Comparison with previous studies

**Table S1.** Comparison with the previous reports on ground state optical absorption/reflection.

| Sample | No. of layers | Temperature (K) | A (eV) | B (eV) | A' (eV) | B' (eV) | IX (eV) | References |
|---|---|---|---|---|---|---|---|---|
| $MoS_2$ | Monolayer | Room | ✓ | ✓ | | | | [20], [22] |
| $MoS_2$ | Few layer, bulk | Room | ✓ | ✓ | | | | [3,22,23] |
| $MoS_2$ | Bilayer | Room | ✓ | ✓ | | | ✓ | [3] |
| $MoS_2$ | Monolayer | Low | ✓ | ✓ | | | | [3] |
| $MoS_2$ | Bi, trilayer | Low | ✓ | ✓ | | | ✓ | [3] |
| $MoS_2$ | Bulk | Low | ✓ | ✓ | | | | [15] |
| $WS_2$ | Monolayer | Room | ✓ | ✓ | | | | [20], [16], [24] |
| $WS_2$ | Few layer | Room | ✓ | ✓ | | | | [23], [16] |
| $WS_2$ | Bulk | Low | ✓ | ✓ | | | | [15] |
| $MoSe_2$ | Monolayer | Room | ✓ | ✓ | | | | [21] |
| $MoSe_2$ | Mono, few layer | Low | ✓ | ✓ | ✓ | ✓ | ✓ | [25], [4] |
| $MoSe_2$ | Bilayer | Low | ✓ | ✓ | | | ✓ | [4] |
| $MoSe_2$ | Bulk | Low | ✓ | ✓ | ✓ | ✓ | ✓ | [15], [4] |
| $WSe_2$ | Monolayer | Room | ✓ | ✓ | ✓ | ✓ | | [16], [21] |
| $WSe_2$ | Few layer | Room | ✓ | ✓ | ✓ | ✓ | | [16] |
| $WSe_2$ | Few layer | Low | ✓ | ✓ | ✓ | ✓ | | [17] |
| $WSe_2$ | Bulk | Low | ✓ | ✓ | ✓ | ✓ | | [15] |
| $MoWS_2$ | Monolayer | Room | ✓ | ✓ | | | | [20] |
| $MoWS_2$ | Few layer | Room | ✓ | ✓ | | | | [23], [26] |
| $MoWS_2$ | Bulk* | Room | ✓ | ✓ | ✓ | ✓ | | *present study |
| $MoWS_2$ | Bulk* | Low | ✓ | ✓ | ✓ | ✓ | ✓ | *present study |
| $MoWSe_2$ | Monolayer | Room | ✓ | ✓ | | | | [21] |
| $MoWSe_2$ | Bulk* | Room | ✓ | ✓ | ✓ | ✓ | ✓ | *present study |
| $MoWSe_2$ | Bulk* | Low | ✓ | ✓ | ✓ | ✓ | ✓ | *present study |

## S2. Structural and compositional properties of bulk alloy single crystals

*X-ray diffraction (XRD):*

Room temperature XRD patterns of bulk $Mo_{0.5}W_{0.5}S_2$ and $Mo_{0.5}W_{0.5}Se_2$ alloy single crystals (procured from HQ Graphene) were recorded using PANalytical 'Empyrean' X-ray diffractometer with Cu Kα radiation (1.54 Å). XRD patterns illustrated in Figs. S1(a,b), revealing the presence of sharp peaks along the *c*-axis (0 0 2*l*), thereby confirming their single crystalline nature.

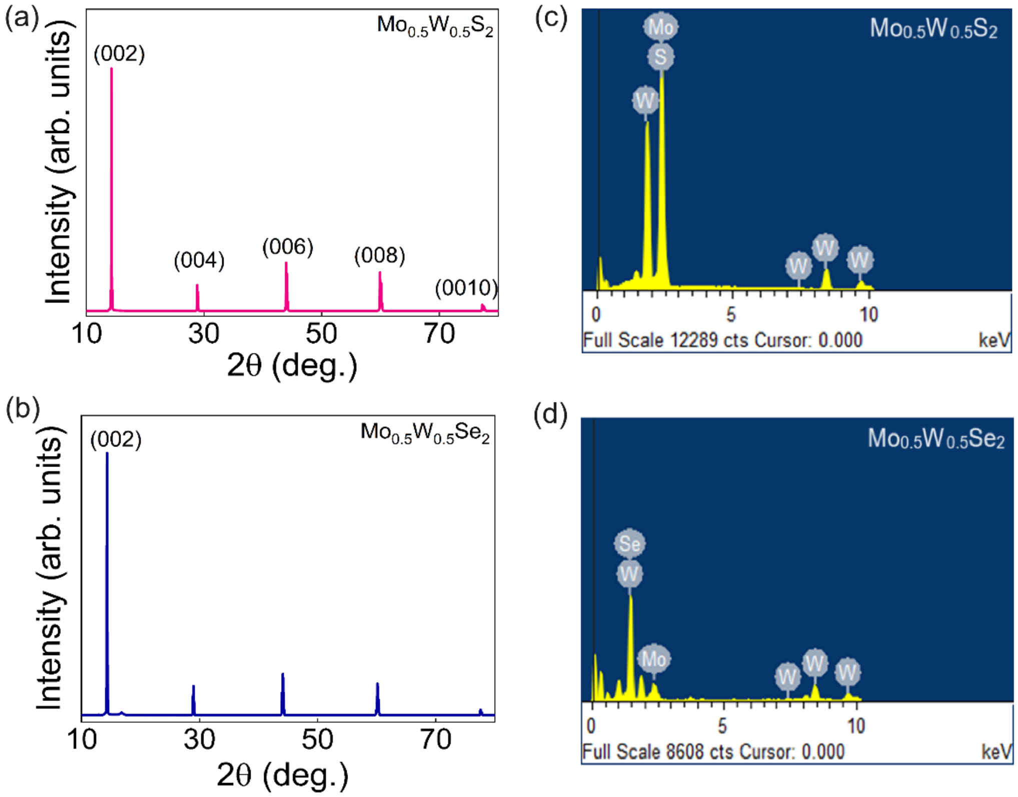


**FIG. S1.** XRD along the c-axis (0 0 2*l*) of bulk (a) $Mo_{0.5}W_{0.5}S_2$ and (b) $Mo_{0.5}W_{0.5}Se_2$ alloy single crystals. (c,d) EDX spectra confirm the uniform distribution of Mo and W with the atomic ratio of Mo:W = 1:1 in both alloys.

*Scanning electron microscopy (SEM) and Energy-dispersive X-ray (EDX) spectroscopy:*

The layered structure of both single crystals was also observed through SEM images (Figs. S2 and S3). To estimate the elemental atomic ratio in bulk $Mo_{0.5}W_{0.5}S_2$ and $Mo_{0.5}W_{0.5}Se_2$ single

crystals, EDX measurements have been done. The overall error estimated in the measurements is less than 1%.

*a) $Mo_{0.5}W_{0.5}S_2$ single crystal:*

EDX were taken from the region marked as pink box in the three SEM images as shown in Fig. S2 and estimated atomic weights of Mo, W, and S are presented in Table S2.

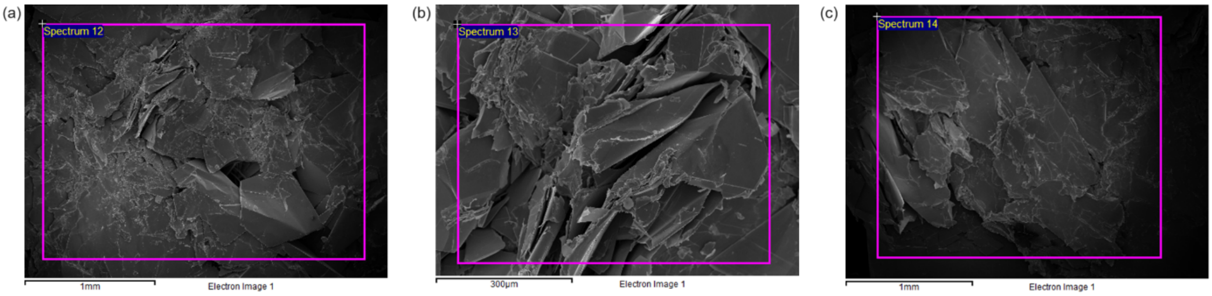


**FIG. S2.** SEM images for bulk $Mo_{0.5}W_{0.5}S_2$ single crystals at three different positions.

**Table S2.** Extracted atomic weight for $Mo_{0.5}W_{0.5}S_2$ single crystal

| Position* | Elements | Weight % | Atomic % |
|---|---|---|---|
| A | S K | 31.40 | 66.65 |
| | Mo L | 23.43 | 16.62 |
| | W M | 45.17 | 16.72 |
| B | S K | 31.76 | 67.03 |
| | Mo L | 23.29 | 16.43 |
| | W M | 44.95 | 16.55 |
| C | S K | 31.39 | 66.60 |
| | Mo L | 23.60 | 16.74 |
| | W M | 45.01 | 16.66 |
| Overall Mo:W = 0.99 ± 0.01 | | | |

*represents positions at different locations in the samples shown in Fig. S2.

*b) $Mo_{0.5}W_{0.5}Se_2$ single crystal:*

EDX were taken from the region marked as pink box in the three SEM images as shown in Fig. S3 and estimated atomic weights of Mo, W, and Se are presented in Table S3.

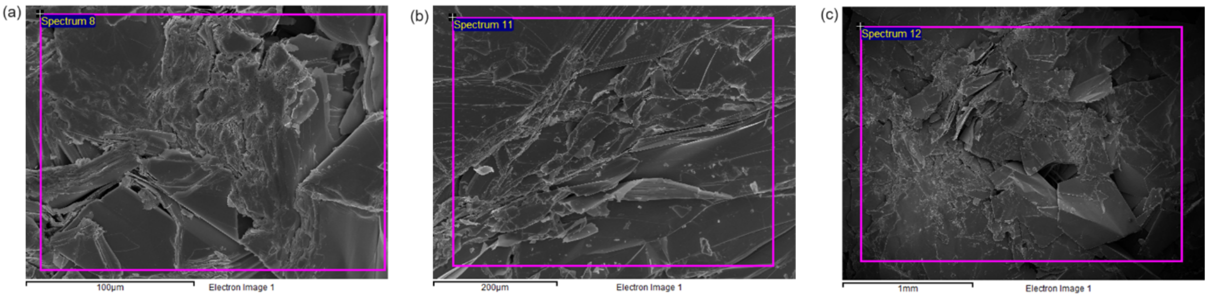


**FIG. S3.** SEM images for bulk $Mo_{0.5}W_{0.5}Se_2$ single crystals at three different positions.

**Table S3.** Extracted atomic weight for $Mo_{0.5}W_{0.5}Se_2$ single crystal

| Position* | Elements | Weight % | Atomic % |
|---|---|---|---|
| A | Se K | 52.87 | 66.73 |
| | Mo L | 15.55 | 16.15 |
| | W M | 31.58 | 17.12 |
| B | Se K | 52.84 | 66.59 |
| | Mo L | 15.89 | 16.48 |
| | W M | 31.27 | 16.92 |
| C | Se K | 52.84 | 66.92 |
| | Mo L | 14.90 | 15.53 |
| | W M | 32.26 | 17.54 |
| Overall Mo:W = 0.93 ± 0.04 | | | |

The EDX spectra confirm the uniform distribution of Mo and W with the atomic ratio of Mo:W = 1:1 in both single crystals.

*X-ray photoemission spectroscopy (XPS):*

Room temperature XPS measurements were carried out using R4000 electron energy analyzer and monochromatic Al Kα ($hv$ = 1486.6 eV) photon source. Single crystals were cleaved in ultra-high vacuum (base pressure was below $5\times10^{-11}$ mbar). The Fermi level and energy resolution of the spectrometer were measured by collecting the Fermi edge spectra of a polycrystalline Ag sample. The total energy resolution was ~300 meV for XPS. The core-level

spectra of Mo, W, S, and Se for both $Mo_{0.5}W_{0.5}S_2$ and $Mo_{0.5}W_{0.5}Se_2$ single crystals are presented in Figs. S4(a,b), respectively. The sharpness of the core-level spectrum of all elements and the absence of additional features, for example, oxide peaks, provide conclusive evidence of the high purity of the single crystals.

The peak assignments with binding energy of all the elements are provided in Tables S4 and S5 for $Mo_{0.5}W_{0.5}S_2$ and $Mo_{0.5}W_{0.5}Se_2$ alloy single crystals, respectively. We have shifted our photoemission spectra to match the experimental valence band and density functional theory (DFT) results (Fig. 1 of the main manuscript), thereby allying the Fermi level at the top of the valence band. Hence, binding energies in the valence band and core level XPS are with respect to the valence band maxima (VBM).

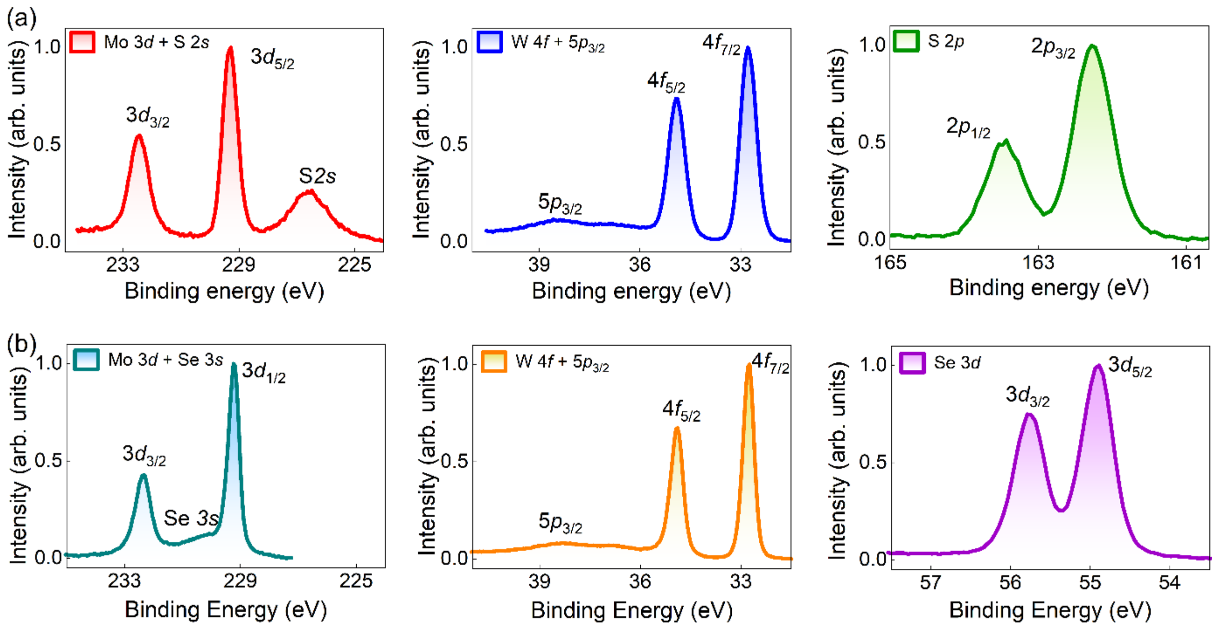


**FIG. S4.** XPS core-level spectrum of bulk (a) $Mo_{0.5}W_{0.5}S_2$ and (b) $Mo_{0.5}W_{0.5}Se_2$ single crystals confirming the high purity of the samples.

**Table S4.** Core-levels of elements with binding energy for $Mo_{0.5}W_{0.5}S_2$ single crystals.

| Elements | Orbitals | Binding energy (eV) |
|---|---|---|
| Mo | $3d_{5/2}$ | 228.6 |
| | $3d_{3/2}$ | 231.7 |
| W | $4f_{7/2}$ | 31.7 |
| | $4f_{5/2}$ | 33.8 |
| | $5p_{3/2}$ | 37.2 |
| S | $2s$ | 225.9 |
| | $2p_{3/2}$ | 161.4 |
| | $2p_{1/2}$ | 162.7 |

**Table S5.** Core-levels of elements with binding energy for $Mo_{0.5}W_{0.5}Se_2$ single crystals.

| Elements | Orbitals | Binding energy (eV) |
|---|---|---|
| Mo | $3d_{5/2}$ | 228.1 |
| | $3d_{3/2}$ | 231.2 |
| W | $4f_{7/2}$ | 32.1 |
| | $4f_{5/2}$ | 34.2 |
| | $5p_{3/2}$ | 37.7 |
| Se | $3s$ | 229.4 |
| | $3d_{5/2}$ | 53.8 |
| | $3d_{3/2}$ | 54.6 |

## S3. Theoretical calculations

*Density functional theory (DFT) calculations:*

Experimental lattice parameters were used for all calculations, and virtual crystal approximation (VCA) [38] was employed to represent the alloy compositions. A plane wave energy cutoff of 400 eV was used, and the effect of SOC was included in all the calculations. Electronic energy was minimized for a $10^{-6}$ eV tolerance, and a Gaussian smearing of 0.05 eV was used. The Brillouin zone was sampled with a 12×12×3 Γ-centered *k*-mesh. Electron energies, initially obtained from PBE calculations, were further refined through single-shot GW ($G_0W_0$) calculations [39,40]. GW optimized pseudopotentials were used for all the calculations and response function cutoff of 266 eV was set for $G_0W_0$. A total of 240 bands, with 52 occupied bands, were considered for comprehensive analysis. The electronic band structures along high symmetry lines were obtained following Wannier interpolation techniques facilitated by the Wannier90 program [41].

*Comparison between virtual crystal approximation (VCA) and supercell method:*

Electronic band structures of bulk $Mo_{0.5}W_{0.5}S_2$ and $Mo_{0.5}W_{0.5}Se_2$ are calculated within VCA [38] and supercell method. In VCA, fractional compositions are considered at the M site, while in the case of the supercell method, a large supercells of a unit cell are used with Mo and W occupying 50% - 50% M sites. The supercell method is computationally expensive and requires a really large supercell to approximate a random distribution of Mo and W in alloy TMDs. Here, we compare the electronic structure calculated within these two methods, VCA (red) and supercell (blue), and show that they provide very similar results. In the supercell method, we chose an ordered structure with 2×2×1 supercell (Fig. S5(a)), and the band structure calculated for the supercell was unfolded in the primitive Brillouin zone. The calculated DFT band structures are presented in Figs. S5(b,c) for bulk $Mo_{0.5}W_{0.5}S_2$ and $Mo_{0.5}W_{0.5}Se_2$, respectively. The band unfolding was performed using the VASPKIT [42] to compare the results of the two

methods. The similarity between the VCA results with the supercell method is clearly seen and justifies the use of VCA for further calculations including many-body $G_0W_0$ and the Bethe-Salpeter equation (BSE).

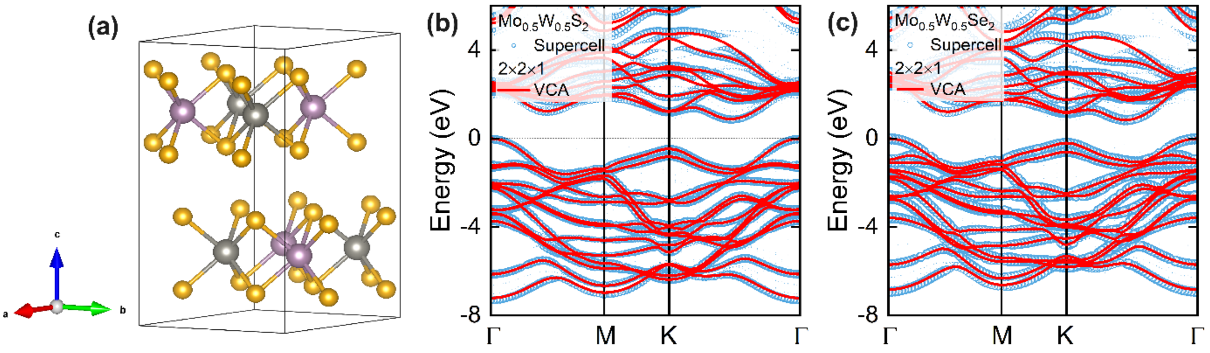


**FIG. S5.** (a) Supercell of 2×2×1 for $Mo_{0.5}W_{0.5}(S/Se)_2$. The grey, purple, and yellow balls represent Mo, W, and S/Se, respectively. Electronic band structure calculated from VCA and supercell methods for bulk (b) $Mo_{0.5}W_{0.5}S_2$ and (c) $Mo_{0.5}W_{0.5}Se_2$.

## S4. Angle-resolved photoemission spectroscopy (ARPES)

To investigate valence band dispersion and spin-orbit coupling (SOC) driven band splitting at K valley, we have performed the ARPES measurements at room temperature using monochromatic He I (*hv* = 21.1 eV) radiation. Single crystal of $Mo_{0.5}W_{0.5}Se_2$ was *in-situ* cleaved. Fig. S6 shows the *k*-resolved band dispersion of $Mo_{0.5}W_{0.5}Se_2$ along $\overline{\Gamma}$-$\overline{K}$ direction. The valence band at $\overline{K}$ point exhibits SOC split bands with a splitting of ~0.37 eV. The spectrum shows weak intensity at the VBM around the $\overline{\Gamma}$ point. The ARPES spectrum was shifted to match to the energies of the top-most energy band, thus aligning the zero energy at the VBM. Constant energy cuts at two different energies, at 0 eV and -0.20 eV integrated within ± 20 meV energy region, are also shown in Fig. S6(c,d). Finite intensity can be seen around $\overline{\Gamma}$ point at 0 eV cut, while for $\overline{K}$ point finite intensity appears at about -0.20 eV cut, suggesting that VBM at $\overline{K}$ point is lower by about 0.20 eV than the global VBM situated at $\overline{\Gamma}$ point. Furthermore, we have included the energy distribution curve from ARPES, clearly showing the SOC splitting of the band of ~0.37 eV at K valley (Fig. S6(d)). The overall band dispersion of $Mo_{0.5}W_{0.5}Se_2$ is similar to that of parent bulk TMDs. The DFT (within VCA) calculated band structure (red line) for $k_z$ = 0.25 (out of plane momentum for He I radiation) overlayed over the ARPES spectrum shows a good agreement, suggesting that DFT is sufficient enough to capture the valence band characteristic in alloys. Notably, in the case of $Mo_{0.5}W_{0.5}S_2$ single crystal, the flake size was smaller than the beam spot size, so we could not acquire reliable data.

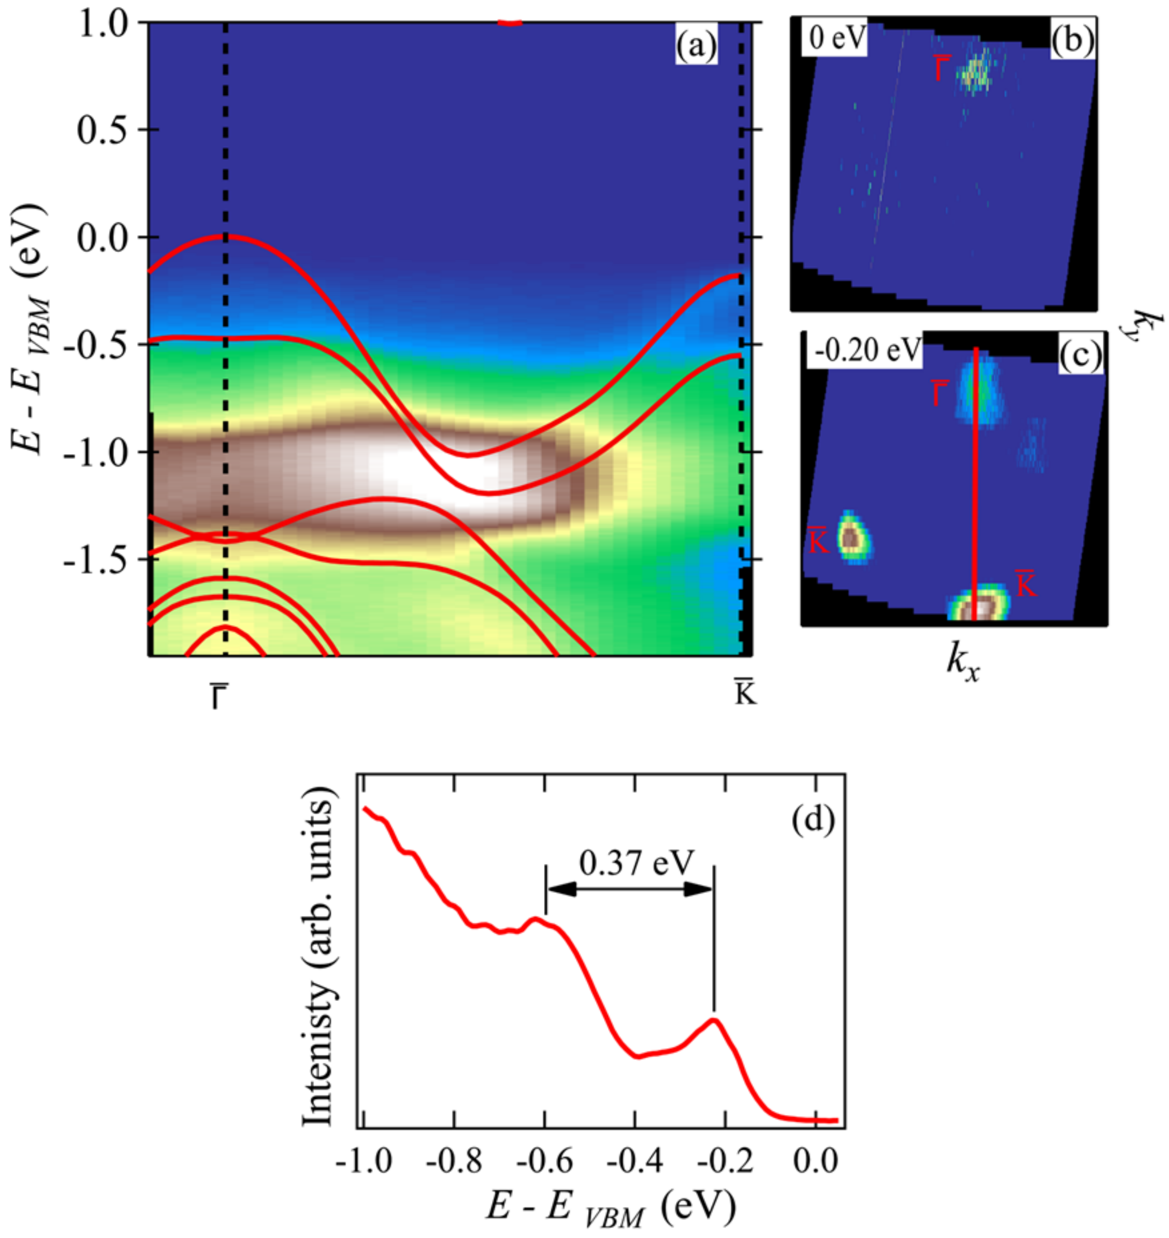


**FIG. S6.** (a) Room temperature ARPES spectrum of $Mo_{0.5}W_{0.5}Se_2$ single crystal collected using He I radiation. DFT VCA calculated band dispersion for $k_z$= 0.25 is represented by red lines. Constant energy cuts at (b) 0 eV and (c) -0.20 eV energies. The red line in (c) shows the cut along which the ARPES spectrum has been shown in (a). (d) Energy distribution curve from ARPES representing the SOC splitting of the band of ~0.37 eV at the K valley.

## S5. Crystal structure

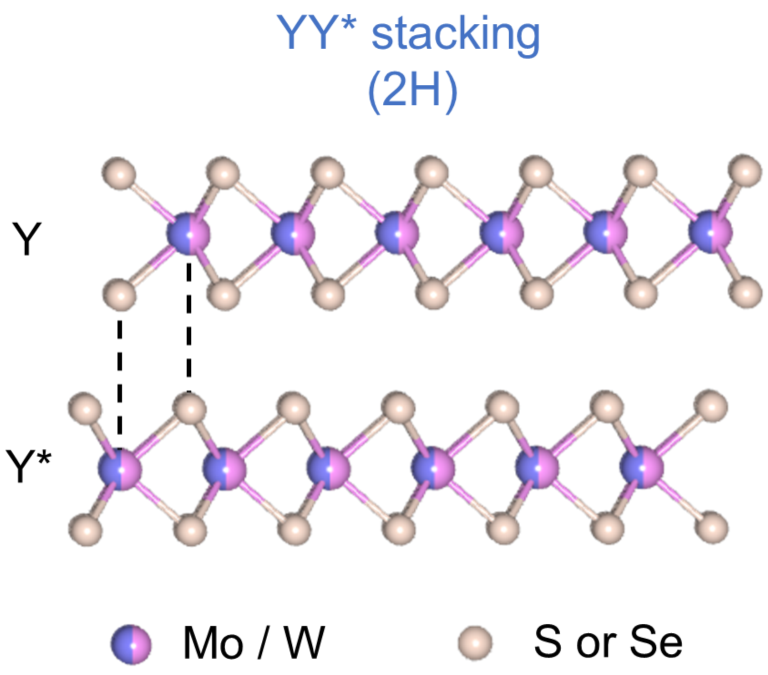


**FIG. S7.** Crystal structure of bulk alloy TMD single crystal representing the 2H phase with YY* stacking. Here, Y consists of trigonal prismatic $MX_6$ arranged in a hexagonal symmetry, while the Y* is 180$^{o}$ in-plane rotated Y stacking.

## S6. Temperature-dependent reflectance spectroscopy

The surface roughness of the sample can affect the scattering of the reflected light; therefore, for correct measurements, a smooth, clean, and shining surface is required. In order to achieve it, both single crystals were cleaved using scotch tape before the measurements. To record the reflected signals, we used a tungsten-halogen lamp as a light source, which offers a broad spectrum in the UV-vis, and near-infrared (1.37-3.54 eV) regions. The sample was mounted in a closed-cycle exchange gas cryostat (Model number: SHI-950-7) at temperatures ranging from 4 to 300 K. The experiments were conducted in a vacuum of ~$10^{-5}$ mbar. A temperature controller is used to change the temperature of the cryostat. Outside the cryostat, the white light was connected to an optical fiber. The experimental setup used in our study is shown in Fig. S8. The beam is steered into the cryostat with the help of mirrors and lenses. The reflected lights are collected using optical fiber and sent to Oceanview spectrometer to record the reflectance spectrum. The experiments on various pieces of samples have been performed multiple times at various positions on the sample surface, and the reproducibility of the results was ascertained.

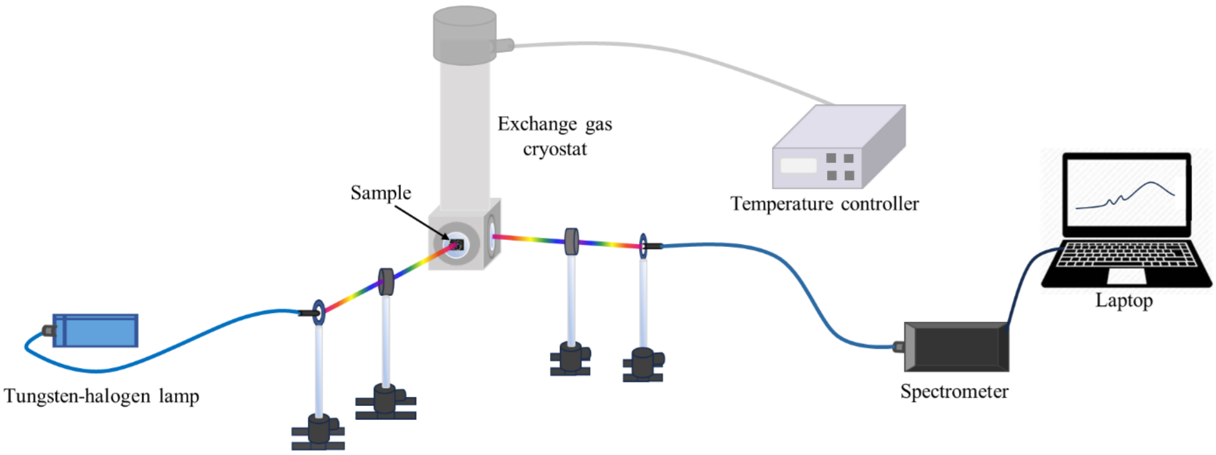


**Fig. S8.** Experimental set-up to measure temperature-dependent reflectance spectroscopy.

### S7. Rydberg excitons in bulk alloy single crystals

*Rydberg excitons in bulk $Mo_{0.5}W_{0.5}S_2$ single crystal:*

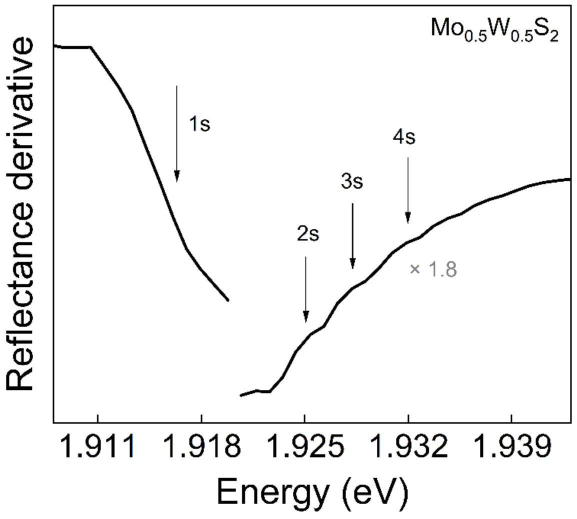


**FIG. S9.** The first derivative of the reflectance spectra calculated from BSE of bulk $Mo_{0.5}W_{0.5}S_2$ single crystal. The arrows represent the exciton Rydberg series up to 4*s* states.

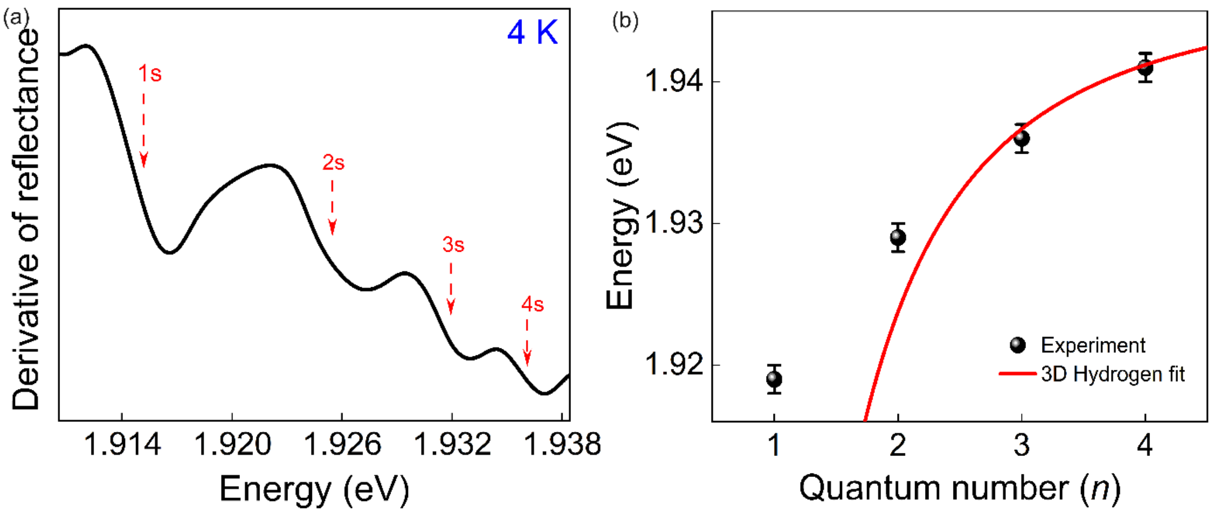


**FIG. S10.** (a) The first derivative of the experimentally measured reflectance spectrum of bulk $Mo_{0.5}W_{0.5}S_2$ single crystal at 4 K. The peaks represent the exciton Rydberg series up to 4*s* states, similar to 80 K data presented in the main manuscript. (b) Experimentally obtained the transition energies of the Rydberg series as a function of quantum number (*n*). The n=3, and 4 peaks follow the 3D hydrogen model and the fit is represented by the red line. The reason for this nonhydrogenic behavior is described in the main manuscript.

## S8. Assignment of A' and B' excitonic transitions

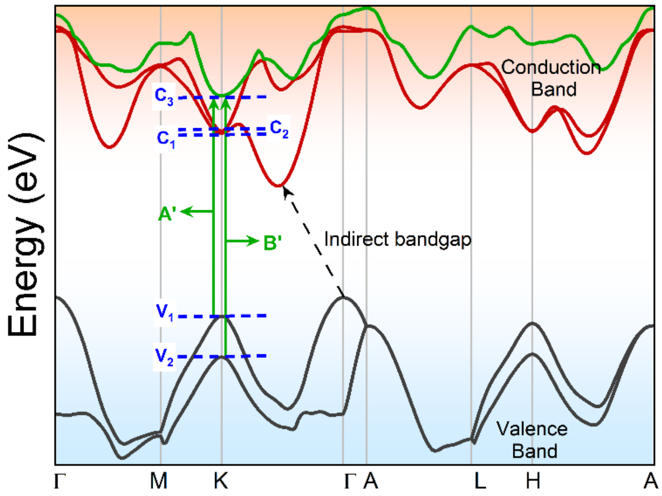


**FIG. S11.** Schematic figure of bulk TMD band structure and various optical transitions, presented here for clarity. The vertical transitions from $V_1^{(\uparrow)} \rightarrow C_3^{(\uparrow)}$, and $V_2^{(\downarrow)} \rightarrow C_3^{(\downarrow)}$ results in the formation A' and B' excitons, respectively. Here, $C_3$ is the spin degenerate band. The assignments of A' and B' excitons are based on experimental observations supported by the electronic band structure.

## S9. Intra and interlayer excitons in TMDs

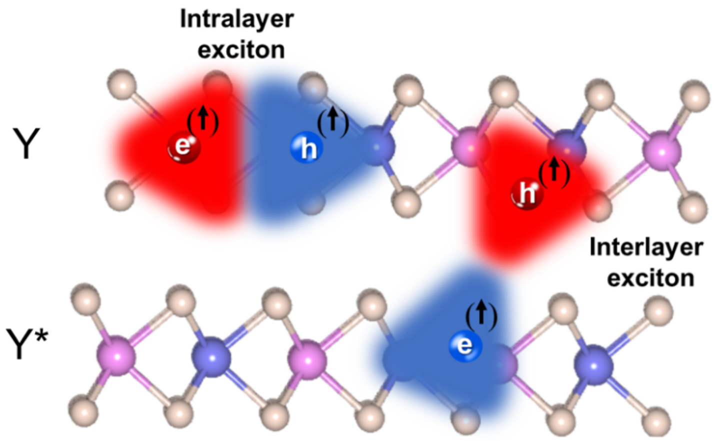


**FIG. S12.** Schematic representation of intralayer and IX excitons in TMDs. Intralayer excitons consist of an electron and a hole in the same layer whereas, for IX, the electron and hole are in different layers. The formation of both excitons is optically allowed only when spins of electron and hole (black arrows) are in the same orientation.

## S10. Calculated absorption spectrum for monolayer alloys

The calculations for monolayers were performed in a similar way as for bulk. We use the same in-plane lattice parameters for the monolayers and the size of the vacuum slab between two adjacent layers was 15 Å. Fig. S13 shows the optical absorption spectra for $Mo_{0.5}W_{0.5}S_2$ and $Mo_{0.5}W_{0.5}Se_2$ monolayers. A and B excitonic features are clearly observed with the splitting of about ~290 and ~330 meV. The excitonic peaks assigned to interlayer excitons (IXs) in the bulk are not found in the monolayers.

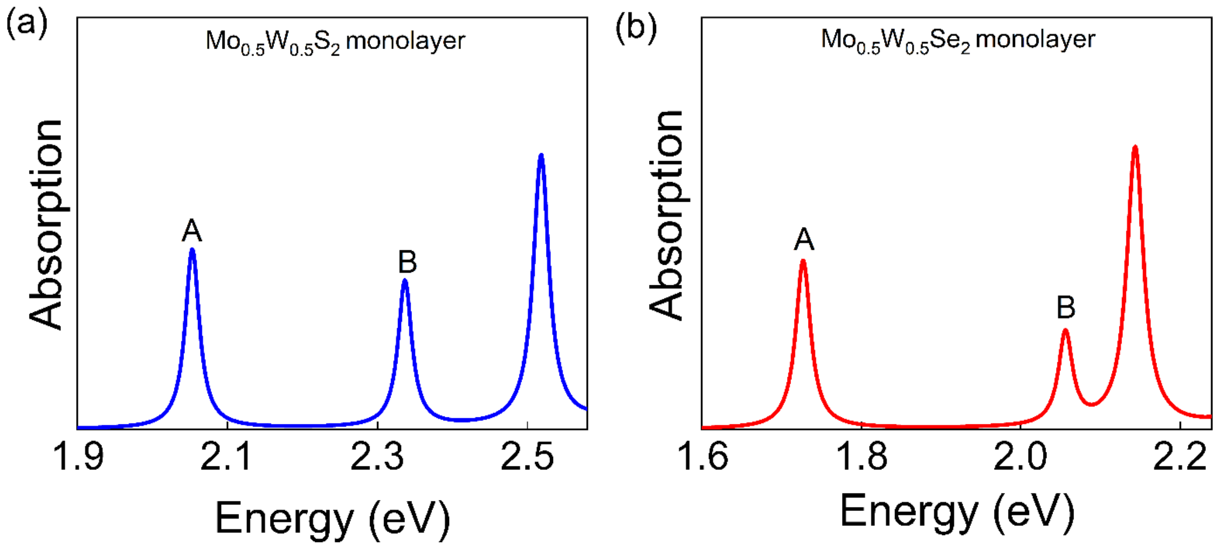


**FIG. S13.** Absorption spectrum obtained from BSE calculations of monolayer (a) $Mo_{0.5}W_{0.5}S_2$ and (b) $Mo_{0.5}W_{0.5}Se_2$. Both spectra show the disappearance of IXs due to absence of interlayer interaction in monolayers.

## S11. Phonon dispersion curves of bulk alloys

Phonon dispersion curves for both systems were calculated for the ordered alloy structure (2×2×1 supercell of the primitive cell) utilizing finite displacement method as implemented in PHONOPY code [59]. A 2×2×2 supercell (total 192 atoms) of the ordered structures with experimental lattice constants was used for phonon calculations. Unfolding of the phonon band structure within the Brillouin zone of the primitive cell was performed using UPHO code [60] and has been shown in Fig. S14. The longitudinal optical phonons appear at ~ 45 meV for $Mo_{0.5}W_{0.5}S_2$ and ~ 32 meV for $Mo_{0.5}W_{0.5}Se_2$ [61].

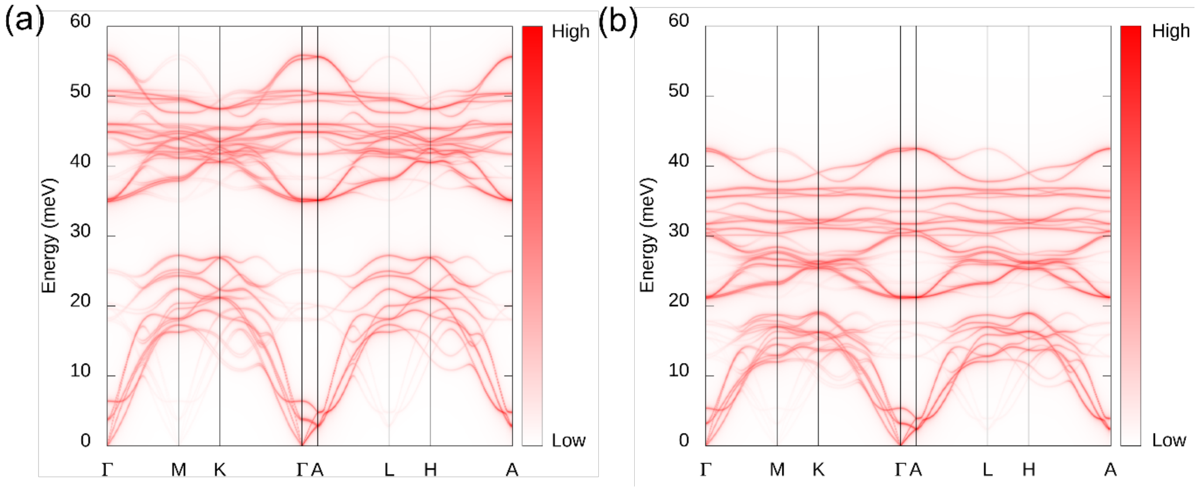


**FIG. S14.** Calculated phonon dispersion curves for bulk (a) $Mo_{0.5}W_{0.5}S_2$ and (b) $Mo_{0.5}W_{0.5}Se_2$.

## References


[3] I. C. Gerber et al., Phys. Rev. B **99**, 035443 (2019).

[4] J. Horng, T. Stroucken, L. Zhang, E. Y. Paik, H. Deng, and S. W. Koch, Phys. Rev. B **97**, 241404 (2018).

[15] A. R. Beal, J. C. Knights, and W. Y. Liang, J. Phys. C: Solid State Phys. **5**, 3540 (1972).

[16] W. Zhao, Z. Ghorannevis, L. Chu, M. Toh, C. Kloc, P. H. Tan, and G. Eda, ACS Nano **7**, 791 (2013).

[17] A. J. Grant, J. A. Wilson, and A. D. Yoffe, Philosophical Magazine **25**, 625 (1972).

[20] A. F. Rigosi, H. M. Hill, K. T. Rim, G. W. Flynn, and T. F. Heinz, Phys. Rev. B **94**, 075440 (2016).

[21] G. Wang et al., Nat Commun **6**, 10110 (2015).

[22] H. Shi, R. Yan, S. Bertolazzi, J. Brivio, B. Gao, A. Kis, D. Jena, H. G. Xing, and L. Huang, ACS Nano **7**, 1072 (2013).

[23] X. Wang, G. Niu, J. Jiang, L. Sui, X. Zeng, X. Liu, Y. Zhang, G. Wu, K. Yuan, and X. Yang, J. Phys. Chem. Lett. **13**, 10395 (2022).

[24] P. D. Cunningham, A. T. Hanbicki, K. M. McCreary, and B. T. Jonker, ACS Nano **11**, 12601 (2017).

[25] A. Arora, K. Nogajewski, M. Molas, M. Koperski, and M. Potemski, Nanoscale **7**, 20769 (2015).

[26] J. Kang, Y. Wang, L. Zhou, O. A. Al-Hartomy, S. Wageh, Y. Wang, H. Zhang, S. Xiao, and J. He, Appl Phys Lett **123**, 061107 (2023).

[38] L. Bellaiche and D. Vanderbilt, Phys. Rev. B **61**, 7877 (2000).

[39] L. Hedin, *New Method for Calculating the One-Particle Green's Function with Application to the Electron-Gas Problem*, Phys. Rev. **139**, A796 (1965).

[40] M. Shishkin and G. Kresse, Phys. Rev. B **74**, 035101 (2006).

[41] A. A. Mostofi, J. R. Yates, Y. S. Lee, I. Souza, D. Vanderbilt, and N. Marzari, Phys Commun **178**, 685 (2008).

[42] V. Wang, N. Xu, J. C. Liu, G. Tang, and W.-T. Geng, *VASPKIT:* Comput Phys Commun **267**, 108033 (2021).

[59] A. Togo, L. Chaput, T. Tadano, and I. Tanaka, J. Phys.: Condens. Matter **35**, 353001 (2023).

[60] Y. Ikeda, A. Carreras, A. Seko, A. Togo, and I. Tanaka, Phys. Rev. B **95**, 024305 (2017).

[61] K. Kaasbjerg, K. S. Thygesen, and K. W. Jacobsen, Phys. Rev. B **85**, 115317 (2012).
